# Supplementary material for: ProtoDepth: Unsupervised Continual Depth Completion with Prototypes
Source: arXiv:2503.12745 source file (2025-03-17)
Supplement: Supplementary file 1 [file X_suppl.tex]

\clearpage
\setcounter{page}{1}
\maketitlesupplementary

\section{Rationale}
\label{sec:rationale}
Having the supplementary compiled together with the main paper means that:
\begin{itemize}
\item The supplementary can back-reference sections of the main paper, for example, we can refer to \cref{sec:intro};
\item The main paper can forward reference sub-sections within the supplementary explicitly (e.g. referring to a particular experiment); 
\item When submitted to arXiv, the supplementary will already included at the end of the paper.
\end{itemize}
To split the supplementary pages from the main paper, you can use \href{https://support.apple.com/en-ca/guide/preview/prvw11793/mac#:~:text=Delete%20a%20page%20from%20a,or%20choose%20Edit%20%3E%20Delete).}{Preview (on macOS)}, \href{https://www.adobe.com/acrobat/how-to/delete-pages-from-pdf.html#:~:text=Choose%20%E2%80%9CTools%E2%80%9D%20%3E%20%E2%80%9COrganize,or%20pages%20from%20the%20file.}{Adobe Acrobat} (on all OSs), as well as \href{https://superuser.com/questions/517986/is-it-possible-to-delete-some-pages-of-a-pdf-document}{command line tools}.

% # download the videos

% # We have csv file for audioset2M
% # Read audioset2M metadata csv

% # make the target directory
% mkdir audioset2m

% # download the videos

% clean_videos

% import os

% def clean_videos(path, split, target_dir):

%     # clip the videos with mm- (apt)

%     # check whether they have audios

%     # save them

%     # save the name on the list
%     return None

% def __main__():

%     # get arguments

%     # Read files (csv or txt)

%     # Create directory for cleaned dataset

%     os.mkdir('audioset2m_clean/video_clean')

%     # Create the list to add the names of cleaned videos

%     # multiprocess - pool~

%     # launch

% process_frames
% import os

% def extract_frames(path, split, target_dir):

%     # extract frames the videos (1 fps) with mm- (apt)

%     # save them

%     # add the name of the file to the txt or csv file

% def __main__():

%     # get arguments

%     # Read files (csv or txt)

%     # Create directory for each frames

%     os.mkdir('audioset2m_clean/frames')
%     for a in range(10):
%         os.mkdir('audioset2m_clean/frames/frame_{}'.format(a))
%     # multiprocess - pool~

%     # launch

% process_audios

% import os

% def extract_audios(path, split, target_dir):

%     # extract audios from the videos with nox (apt)

%     # save them

%     # add the name of the file to the txt or csv file

% def __main__():

%     # get arguments

%     # Read files (csv or txt)

%     # Create directory for cleaned dataset

%     os.mkdir('audioset2m_clean/audio')
%     # multiprocess - pool~

%     # launch
